# Supplementary material for: Trackable Island-model Genetic Algorithms at Wafer Scale
Source: arXiv:2405.03605 source file (2024-05-06)
Supplement: Supplementary file 1 [file supplement.tex]

\section{Application Form Questions}

\subsection{Project Title}

Characterization of Phylogenetic Structure Across Population Scales using Wafer-scale Agent-based Evolution Simulation

\subsection{Public overview}

\begin{displayquote} \itshape
Your overview should touch on your project's goals, how you plan to use ACCESS resources, and any software packages you need.
Covering these topics helps us ensure you get connected with appropriate resources for your work.
\end{displayquote}

% Large-scale evolutionary processes underlie key problems in .
Cross-scale dynamics of large-scale evolutionary processes underly key questions in evolutionary biology, public health, medicine, and natural resources management.
Understanding the dynamics of vast, evolving populations can help address challenges like communicable disease, antibiotic resistance, cancer treatment, and conservation biology, as well as addressing scientific questions related to ecological communities and evolutionary transitions in individuality (e.g., multicellularity).
Emerging massively parallel hardware accelerators have immense potential to provide the extensive computation necessary to advance simulation experiments investigating these phenomena.
However, critical methodological gaps prevent effective application of these accelerators to evolution simulations.
Phylogenetic records (i.e., the history of evolutionary relatedness among organisms) are needed to fully understand the mode and tempo of evolution within simulated populations.
However, existing phylogenetic tracking techniques are poorly aligned to new accelerators' highly distributed, many-processor architectures.

Recently introduced hereditary stratigraphy algorithms provide a potential solution to collect phylogenetic data from large-scale in silico evolution experiments.
These algorithms annotate simulated genomes with heritable markers that, after simulation ends, facilitate inference of phylogenetic history among end-state evolved agents.
Our project builds on promising pilot work with hereditary stratigraphy algorithms, taking first steps to assess these algorithms' capabilities and limitations at scale on the Cerebras Wafer Scale Engine, a leading example of cutting-edge accelerator technology.
As a case study, we will use tracking-enabled simulation to investigate fundamental questions about how the phylogenetic structure of natural systems is influenced by orders-of-magnitude differences in population size.

Work will unfold in three phases:
1. Algorithm Validation: compare replicate evolutionary runs across selection pressure levels, and evaluate the capability of hereditary stratigraphy to detect expected effects on phylogenetic structure in wafer-scale agent populations;
2. Scalability Analysis: assess stability, efficiency, and throughput of tracking-enabled simulation in processor collections ranging from hundreds, to thousands, to full wafer scale; and
3. Phylogenetic Structure Across Population Scales: exploit wafer-scale computation to assess how commonly measured aspects of phylogenetic structure vary with scale in generational depth and population size.

Evaluated methods promise to enable currently intractable computational research, benefiting further explorations of evolutionary processes impacting public health, medicine, and beyond.
Our project aims not only to shed light on fundamental questions about how aspects of phylogenetic structure emerge from evolutionary processes, but also to open new frontiers in what's possible for digital evolution research.

\subsection{Keywords}

agent-based modeling, digital evolution, genetic algorithms, phylogenetics, evolutionary biology

\subsection{Fields of Science}

\begin{enumerate}
    \item Systems and Population Biology
    \item Other Computer and Information Sciences
\end{enumerate}

\subsection{How many CS-2 hours are requested? Provide comments.}

80 hours

We anticipate that between a half hour and a full hour of compute time for each replicate will be sufficient to observe very deep evolutionary processes (i.e., on the order of a million generations).
We estimate 10 hours for validation experiments and 30 hours for our main experiments exploring interactions between population scale and phylogenetic structure.

We have budgeted 20 hours of compute time for scale-up benchmarking experiments.
We estimate 20 minutes of runtime likely sufficient per replicate, and plan 20 replicates per each of our 3 scale treatments.

An additional 20 hours are included to account for debugging, testing, and any unforeseen circumstances.

\subsection{Mow much storage space is requested? Please, describe your data format and size in GB. Make sure to request as many GB of PSC Bridges-2 Ocean storage.}

2000GB, CSV and Parquet files containing agent genomes and phylogenetic reconstructions

Due to the CS-2 device's 44 GB of onboard memory, exporting the full end-state of an evolutionary simulation from the WSE hardware would occupy less than 50GB.
Thus, a 1000 GB capacity would allow us to store data from at least 40 replicate experiments.
We expect the storage footprint of reconstructed phylogenies to be no more than the size of the raw agent genome data, and allocate an additional 1000 GB for that purpose.

Although later experiments may stream sampled agent genomes off of the device during runtime, we anticipate collecting no more than hundreds of GB of such data.

\subsection{Describe your research team.}

\begin{displayquote} \itshape
Please, describe your research team and make sure to include expected roles in the proposed research, current affiliation, academic status, and relevant experience.
Links to professional pages or attached documents that describe relevant experience and qualifications are welcomed.
\end{displayquote}

The lead researcher on this project is Dr. Matthew Andres Moreno.
Dr. Moreno is a postdoctoral researcher at University of Michigan with affiliations with the Ecology and Evolutionary Biology Department, the Center for the Study of Complex Systems, and the Michigan Institute for Data Science.
His work is supported through the Schmidt AI in Science postdoctoral fellowship.

Dr. Moreno gained extensive experience in software engineering for scientific software during his graduate training, with a special emphasis on parallel/distributed computing.
Application of high-performance computing for digital evolution simulation has since become an ongoing theme of Dr. Moreno's research.
In addition to his current work on decentralized phylogenetic tracking, he has also investigated application of asynchronous and best-effort computing strategies for scalable simulations of evolving digital multicells.
These projects led to the development of the hstrat and dishtiny/conduit software libraries, respectively, which can be found on his GitHub profile at \url{https://github.com/mmore500/}.
He has also been active in training and mentoring activities within the scientific computing and software development communities, notably serving as the lead organizer for the Workshop for Avida-Ed Software Development (WAVES) research experience for undergraduates program in 2020 and 2021.
Training materials and capstone projects from the workshop can be viewed at \url{https://mmore500.com/waves}.
More information about Dr. Moreno's research can be found at \url{https://mmore500.com/research/}.

Dr. Emily Dolson and Dr. Luis Zaman are close collaborators, taking on an advisory role in this project.

Dr. Zaman is an assistant professor at University of Michigan with affiliations to Ecology and Evolutionary Biology and the Center for the Study of Complex Systems.
The ZE3 lab studies host-parasite co-evolution dynamics.
In addition to work with benchtop experiments involving bacteria and phage models, Dr. Zaman has extensive experience harnessing the simulation tools like the Avida Digital Evolution platform to conduct sophisticated \textit{in silico} experiments.
Dr. Zaman serves as Dr. Moreno's postdoctoral advisor.

Dr. Emily Dolson is an assistant processor at Michigan State University, primarily affiliated to the Computer Science and Engineering department.
She is also affiliated with the Ecology, Evolution, and Behavior program.
A leading theme of Dr. Dolson's ongoing work is incorporation of phylogenetic methods into digital evolution work, with specific projects focusing on diagnostics for application-oriented evolutionary algorithms and characterization of open-ended evolutionary dynamics with artificial life systems, among other areas.
Her work incorporates special focus on biomedical applications for developed techniques to assess and manipulate evolutionary dynamics, drawing from her oncology-focused postdoctoral training at the Cleveland Clinic.
Dr. Dolson also brings an extensive software engineering background to the project.
Among other software contributions, she led development of extensive phylogenetic tracking tools for the Empirical C++ library.
This project can be viewed at \url{https://github.com/emilydolson/phylotrackpy}.

Undergraduate researchers Connor Yang and Anika Ranjan are involved in the project through the Undergraduate Research Opportunities Program at University of Michigan.
Connor's primary role is in software development, including contributing Cerebras Software Language code to be used in the project.
Anika's role has been in data analysis for experiments testing the algorithmic properties of hereditary stratigraphy approaches.
Both undergraduate students work under the supervision of Dr. Moreno.

\subsection{Which Neocortex Application Track?}

Track 3: General purpose SDK

\begin{displayquote} \itshape
This track is for researchers who intend to leverage the Cerebras SDK to develop custom compute kernels.
The SDK is for researchers who want to explore the fundamental mapping of algorithms to a gigantic rectangular mesh of independent processors with a unique memory architecture.
Ongoing research work with the SDK includes a collaboration with an energy company to implement a finite difference method for seismic wave equations and the implementation of Graph 500 benchmark algorithms.

Some potential research avenues of interest are the implementation of HPC benchmark algorithms, such as HPL (high-performance LINPACK) and HPCG (high-performance conjugate gradient), optimal mappings of sparse tensor operations, linear solvers, particle methods, or graph algorithms, for instance.

The SDK can also be used to explore the implementation of custom machine learning kernels on the CS-2.
Note however, that the SDK is not currently interoperable with the CS-2's PyTorch and TensorFlow frontends, and can only be used to write standalone code.
Also, note that existing code written in other languages cannot be used as-is.

To better understand what leveraging the SDK entails, it can be helpful to envision what CUDA development would look like for a specific GPU architecture.
\end{displayquote}

\subsection{Did you address all the questions associated with the track(s) in an attached application PDF document?}

\begin{displayquote} \itshape
    \begin{itemize}
    \item \url{https://portal.neocortex.psc.edu/docs/index.html}
    \item \url{https://www.cmu.edu/psc/aibd/neocortex/2023-11-neocortex-project-tracks.html}
    \end{itemize}
\end{displayquote}

\begin{displayquote} \itshape
    \begin{enumerate}
    \item Using the SDK requires programming in CSL, a C-like language designed specifically for the problem of massively parallel programming on the CS-2.
    What is your experience with HPC programming paradigms and languages, such as MPI, OpenMP, CUDA, OpenCL, etc.?
    \item What are the underlying computational algorithms you're interested in exploring?
    What existing software packages or libraries use these algorithms?
    \item How is this problem bottlenecked on current hardware?
    Is the problem more bottlenecked by memory bandwidth, or communication costs associated with scaling up across distributed compute nodes?
    \item What range of problem sizes are you interested in addressing?
    For example, how much memory does your problem use?
    How does memory usage or program run-time scale with problem size?
    \item What portion of your algorithm do you plan to port to the CS-2?
    Why are you interested in exploring this part of your algorithm?
    \item The CS-2 offers native half and single precision data types.
    What precision does your algorithm or use case need?
    \item The CS-2 is a network-attached accelerator. At a high level, the CSL programming model is similar to that of CUDA, in which data is moved between host CPU nodes and the device (CS-2) on which computational kernels are launched.
    How often will data need to be moved between the wafer and the worker nodes?
    \item Describe your general plan to map your problem onto 850,000 cores. In answering this question, it might be helpful to recall some details of the CS-2 architecture.
    The 850,000 cores are laid out in a mesh, with each core connected on fabric to its four nearest neighbors on the East, South, North, and West.
    Memory is distributed among the cores, with each core having 48 KB of local memory.
    64-bit local memory reads and writes take roughly a cycle, as does sending and receiving 32-bit messages between the four neighboring cores.
    \end{enumerate}
\end{displayquote}
