# Supplementary material for: Trackable Island-model Genetic Algorithms at Wafer Scale
Source: arXiv:2405.03605 source file (2024-05-06)
Supplement: Supplementary file 3 [file supplement.tex]

\section{Supplemental Material}

% Define lighter colors
\definecolor{LighterBlue}{rgb}{0.84, 0.92, 0.95}
\definecolor{LighterSalmon}{rgb}{1.0, 0.81, 0.76}
\definecolor{LighterPastelGreenYellow}{rgb}{0.88, 0.96, 0.90}

% Define thick vertical lines for section dividers
\newcolumntype{q}{!{\color{white} \vrule width 2pt}}

\begin{figure*}
    \centering
\begin{minipage}[t]{\textwidth}
\centering
\footnotesize
\begin{tabular}{
c
>{\columncolor{LighterBlue}}c
>{\columncolor{LighterBlue}}c
>{\columncolor{LighterSalmon}}c
>{\columncolor{LighterSalmon}}c
q % Thick divider
>{\columncolor{LighterPastelGreenYellow}}c
>{\columncolor{LighterPastelGreenYellow}}c
>{\columncolor{LighterPastelGreenYellow}}c
>{\columncolor{LighterPastelGreenYellow}}c
q % Thick divider
>{\columncolor{LighterPastelGreenYellow}}c
>{\columncolor{LighterPastelGreenYellow}}c
>{\columncolor{LighterPastelGreenYellow}}c
>{\columncolor{LighterPastelGreenYellow}}c
}
& \multicolumn{4}{cq}{\cellcolor{white}Word 0} & \multicolumn{4}{cq}{\cellcolor{white}Word 1} & \multicolumn{4}{c}{\cellcolor{white}Word 2} \\
\cmidrule(l{1.5pt}r{1.5pt}){2-5}
\cmidrule(l{1.5pt}r{1.5pt}){6-9}
\cmidrule(l{1.5pt}r{1.5pt}){10-13}
Byte & {\cellcolor{white}0} & {\cellcolor{white}1} & {\cellcolor{white}2} & {\cellcolor{white}3} & {\cellcolor{white}4} & {\cellcolor{white}5} & {\cellcolor{white}6} & {\cellcolor{white}7} & {\cellcolor{white}8} & {\cellcolor{white}9} & {\cellcolor{white}10} & {\cellcolor{white}11} \\
\cmidrule(l{1.5pt}r{1.5pt}){2-2}
\cmidrule(l{1.5pt}r{1.5pt}){3-3}
\cmidrule(l{1.5pt}r{1.5pt}){4-4}
\cmidrule(l{1.5pt}r{1.5pt}){5-5}
\cmidrule(l{1.5pt}r{1.5pt}){6-6}
\cmidrule(l{1.5pt}r{1.5pt}){7-7}
\cmidrule(l{1.5pt}r{1.5pt}){8-8}
\cmidrule(l{1.5pt}r{1.5pt}){9-9}
\cmidrule(l{1.5pt}r{1.5pt}){10-10}
\cmidrule(l{1.5pt}r{1.5pt}){11-11}
\cmidrule(l{1.5pt}r{1.5pt}){12-12}
\cmidrule(l{1.5pt}r{1.5pt}){13-13}
& \multicolumn{4}{cq}{\cellcolor{white}} & \multicolumn{4}{cq}{\cellcolor{white}} & \multicolumn{4}{c}{\cellcolor{white}} \\[-2ex]
\scriptsize{Genome 0} & \texttt{F9} & \texttt{02} & \texttt{79} & \texttt{00} & \texttt{8D} & \texttt{22} & \texttt{4F} & \texttt{F3} & \texttt{D2} & \texttt{78} & \texttt{AD} & \texttt{C7} \\
& \multicolumn{4}{cq}{\cellcolor{white}} & \multicolumn{4}{cq}{\cellcolor{white}} & \multicolumn{4}{c}{\cellcolor{white}} \\[-2ex]
\scriptsize{Genome 1} & \texttt{F9} & \texttt{02} & \texttt{75} & \texttt{00} & \texttt{8D} & \texttt{A1} & \texttt{CB} & \texttt{F2} & \texttt{D1} & \texttt{5B} & \texttt{CC} & \texttt{D4} \\
& \multicolumn{4}{cq}{\cellcolor{white}} & \multicolumn{4}{cq}{\cellcolor{white}} & \multicolumn{4}{c}{\cellcolor{white}} \\[-2ex]
\scriptsize{Genome 2} & \texttt{61} & \texttt{B6} & \texttt{65} & \texttt{00} & \texttt{66} & \texttt{29} & \texttt{B4} & \texttt{F0} & \texttt{62} & \texttt{99} & \texttt{5A} & \texttt{61} \\
{\cellcolor{white}\ldots} & {\cellcolor{white}\ldots} & {\cellcolor{white}\ldots} & {\cellcolor{white}\ldots} & {\cellcolor{white}\ldots} & {\cellcolor{white}\ldots} & {\cellcolor{white}\ldots} & {\cellcolor{white}\ldots} & {\cellcolor{white}\ldots} & {\cellcolor{white}\ldots} & {\cellcolor{white}\ldots} &
{\cellcolor{white}\ldots} & {\cellcolor{white}\ldots} \\
\end{tabular}
\end{minipage}

\begin{minipage}[t]{\textwidth}
\caption{%
\textbf{Example genomes sampled after validation experiment completion.}
  In validation testing, genomes were composed of three 32-bit words.
  The first two bytes (blue) are fixed random markers generated at simulation start-up, indicating independent lineage originations.
  The next two bytes (salmon) are a generation counter.
  Bits within the final eight bytes are lineage checkpoint values to facilitate phylogenetic reconstruction, arranged according to a tilted hereditary stratigraphic algorithm.
  Note that this genome does not include any content affecting agent traits or fitness --- neutral selection was used for this validation experiment.
}
\label{fig:genome-layout}
\end{minipage}
\end{figure*}
