# Supplementary material for: Trackable Island-model Genetic Algorithms at Wafer Scale
Source: arXiv:2405.03605 source file (2024-05-06)
Supplement: Supplementary file 4 [file supplement.tex]

\section{Supplemental Material}

\section{Example} \label{sec:example}

example \citep{gropp1996high}
