# Supplementary material for: Trackable Island-model Genetic Algorithms at Wafer Scale
Source: arXiv:2405.03605 source file (2024-05-06)
Supplement: Supplementary file 7 [file build-tree-trie-implementation.tex]

\subsection{Trie-based Phylogenetic Tree Reconstruction Implementation}

This section provides source code and docstrings for trie-based phylogeny reconstruction.

The main reconstruction logic takes place in \texttt{build\_trie\_from\_artifacts} (Listing \ref{lst:build_tree_from_artifacts}).
First, hereditary stratigraphic annotations associated with each extant population member are sorted by the generational depth of their lineages in ascending order.
This ensures that higher-per-generation-density hereditary stratigraphic records of annotations from shorter lineages are encountered first.
(In this work, because generations are synchronous, this step had no effect.)

Next, annotations are inserted into a trie data structure one at a time.
All annotations begin at the root node of the trie, representing a universal common ancestor.
Each subsequent node in the trie denotes a particular ``fingerprint'' value associated with its generation of creation.
(This is referred to in the source code as an ``allele'').
Paths traced from the root node towards the tips therefore represent a particular sequence of allele generation events; organisms will share common allele generation histories for the over the evolutionary interval they share common ancestry.

Each annotation descends the trie along the path corresponding to the sequence of alleles contained within its own record.
The \texttt{GetDeepestCongruousAllele} member function of the \texttt{TrieInnerNode} class implements this process.
When no further consistent alleles are present in the trie, the remaining alleles within the annotation are unrolled to create a new unifurcating branch.
The label corresponding to the annotation is then appended as the leaf node on that branch.
The \texttt{InsertTaxon} member function of the \texttt{TrieInnerNode} class implements this process.
The \texttt{TrieInnerNode} and \texttt{TrieLeafNode} classes are provided in Listings \labelcref{lst:TrieInnerNode,lst:TrieLeafNode}.

The \texttt{build\_tree\_trie} method (Listing \ref{lst:build_tree_trie}) serves as the API entrypoint for the overall tree reconstruction routine.
Default options were used for all reconstructions in this work.
The \texttt{build\_tree\_trie} entrypoint delegates to \texttt{build\_tree\_trie\_ensemble} (Listing \ref{lst:build_tree_trie_ensemble}), which ultimately delegates to \texttt{build\_build\_trie\_from\_artifacts}.
These additional source files are included due to docstring parameter descriptions referenced in other files and information about minor trie postprocessing performed to perform ancestor origin time estimates and convert the trie structure into a standard phylogenetic output format.
Listing \ref{lst:AssignOriginTimeNaiveTriePostprocessor} provides the particular postprocessing implementation used to estimate ancestor origin times in reconstructions performed as part of this work.

The full source context for the files included in listings can be found at \url{https://github.com/mmore500/hstrat}.

\lstinputlisting[
  language=Python,
  label={lst:build_tree_from_artifacts},
  caption={\texttt{\_build\_trie\_from\_artifacts.py} source code},
  style=mypython
]{hstrat/hstrat/phylogenetic_inference/tree/_impl/_build_trie_from_artifacts.py}

\lstinputlisting[
  language=Python,
  label={lst:TrieInnerNode},
  caption={\texttt{\_TrieInnerNode.py} source code},
  style=mypython
]{hstrat/hstrat/phylogenetic_inference/tree/_impl/_TrieInnerNode.py}

\lstinputlisting[
  language=Python,
  label={lst:TrieLeafNode},
  caption={\texttt{\_TrieLeafNode.py} source code},
  style=mypython
]{hstrat/hstrat/phylogenetic_inference/tree/_impl/_TrieLeafNode.py}

\lstinputlisting[
  language=Python,
  label={lst:build_tree_trie},
  caption={\texttt{\_build\_tree\_trie.py} source code},
  style=mypython
]{hstrat/hstrat/phylogenetic_inference/tree/_build_tree_trie.py}

\lstinputlisting[
  language=Python,
  label={lst:build_tree_trie_ensemble},
  caption={\texttt{\_build\_tree\_trie\_ensemble.py} source code},
  style=mypython
]{hstrat/hstrat/phylogenetic_inference/tree/_build_tree_trie_ensemble.py}

\lstinputlisting[
  language=Python,
  label={lst:AssignOriginTimeNaiveTriePostprocessor},
  caption={\texttt{\_AssignOriginTimeNaiveTriePostprocessor.py} source code},
  style=mypython
]{hstrat/hstrat/phylogenetic_inference/tree/trie_postprocess/_AssignOriginTimeNaiveTriePostprocessor.py}
