# Supplementary material for: Trackable Island-model Genetic Algorithms at Wafer Scale
Source: arXiv:2405.03605 source file (2024-05-06)
Supplement: Supplementary file 8 [file supplement.tex]

\section{Supplemental Material}

\input{fig/genome-layout}
